# Supplementary material for: Contextual Budget Bandit for Food Rescue Volunteer Engagement
Source: arXiv:2509.10777 source file (2025-09-13)

# Synthetic Food Rescue Data

Reward

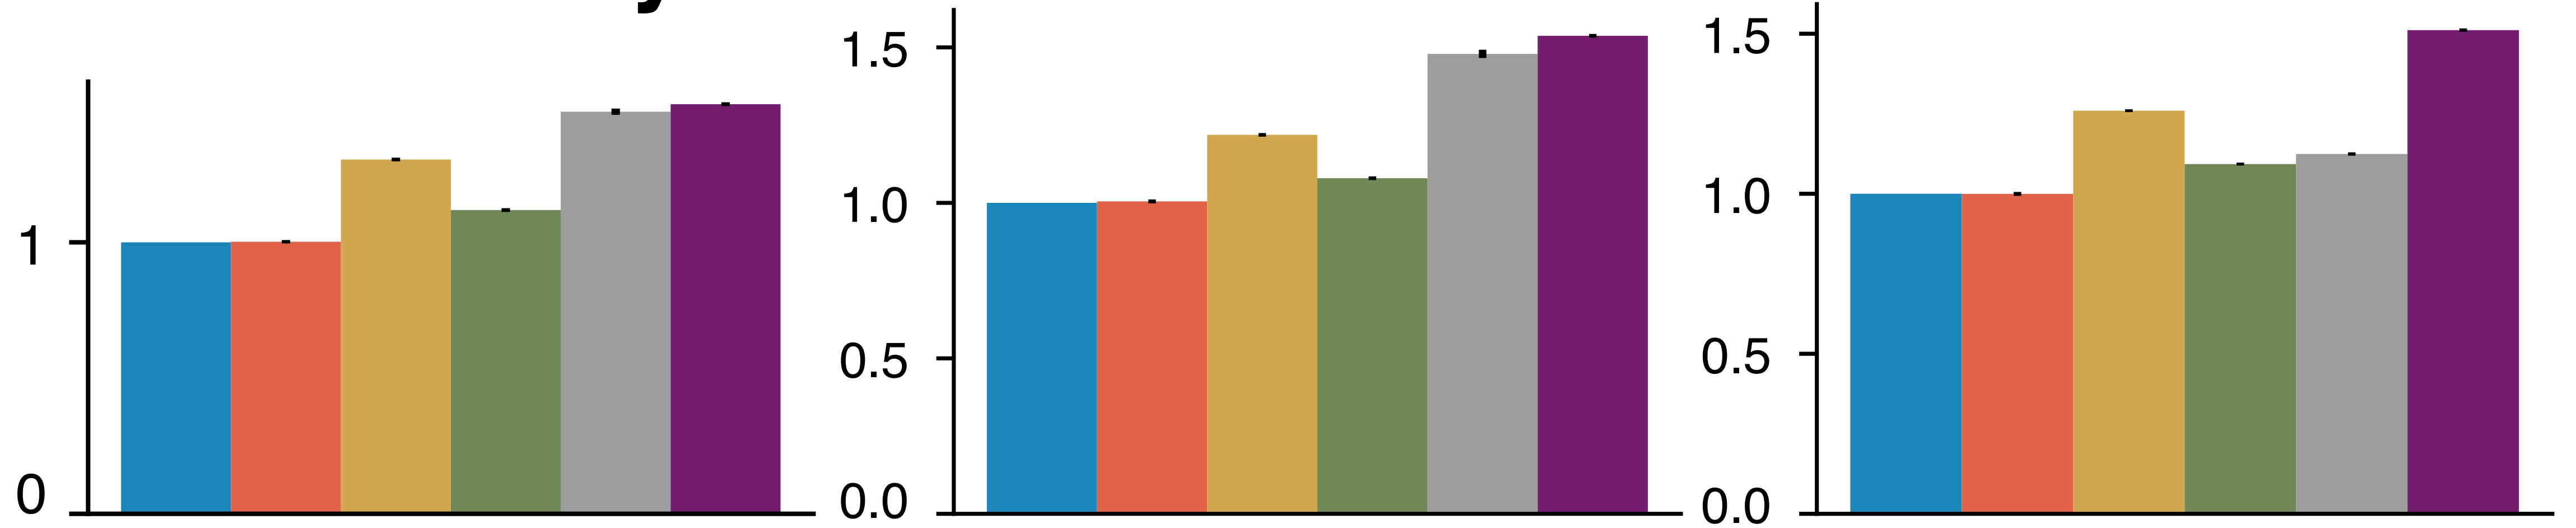

Time

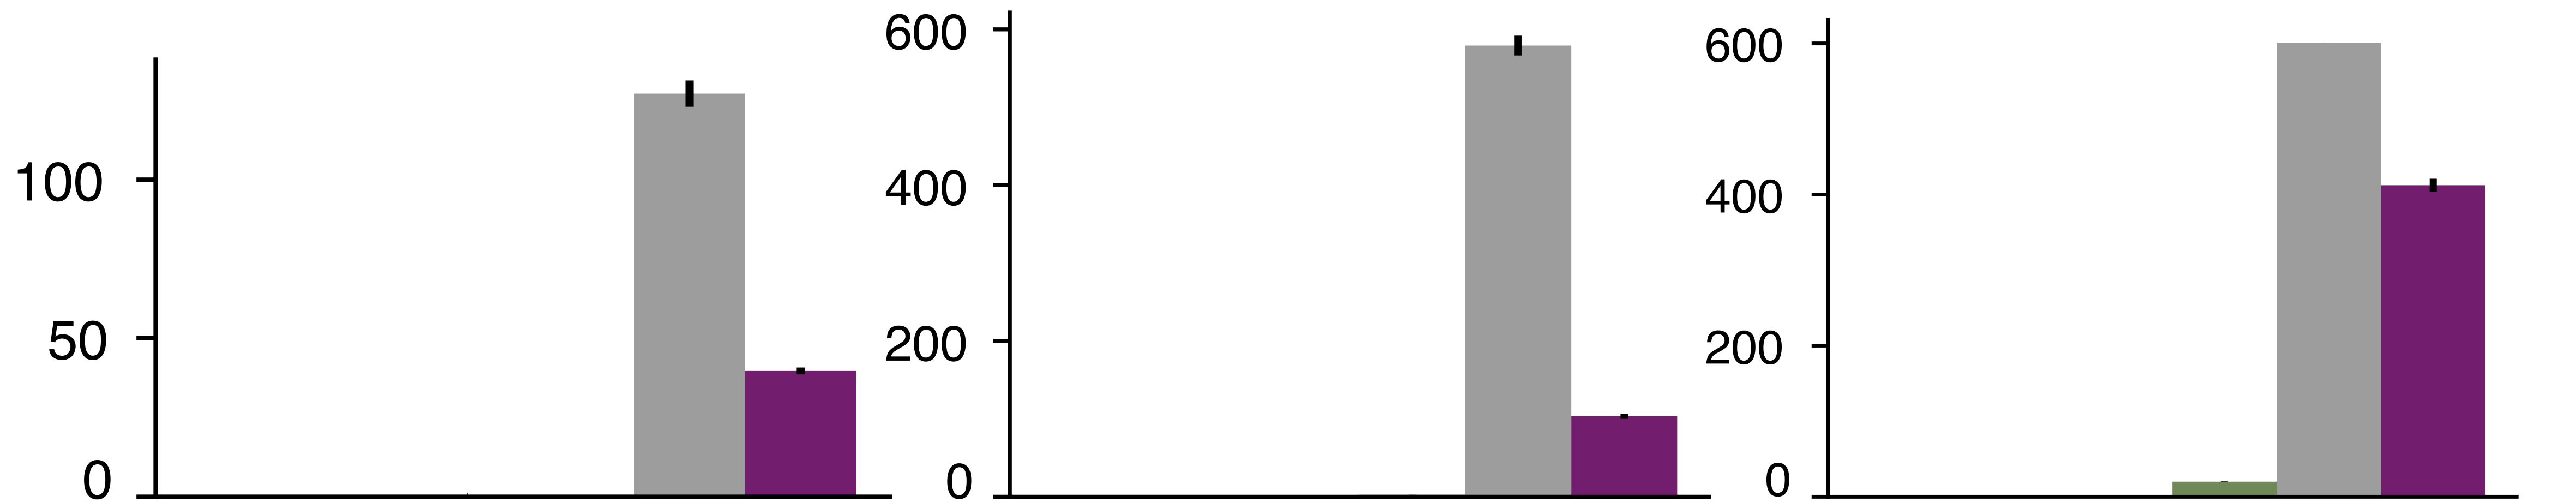

K=3

K=4

K=5

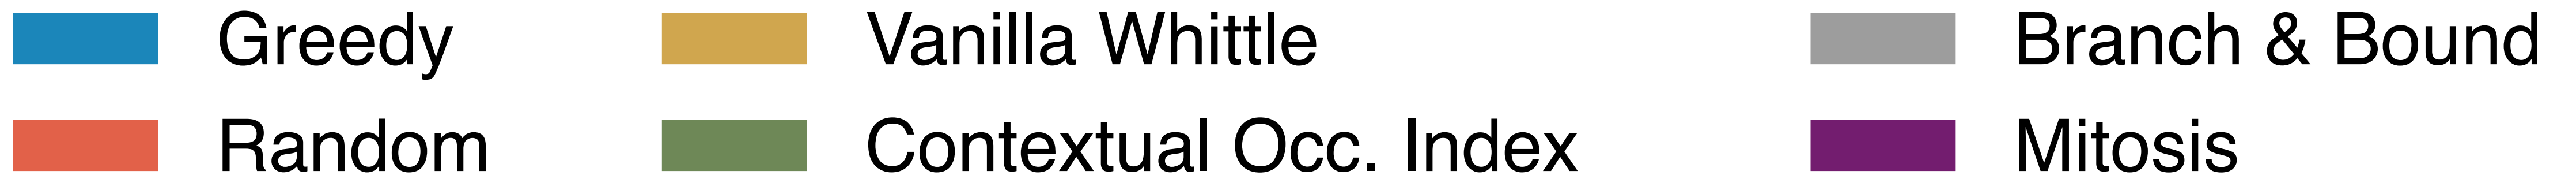

# Real Food Rescue Data

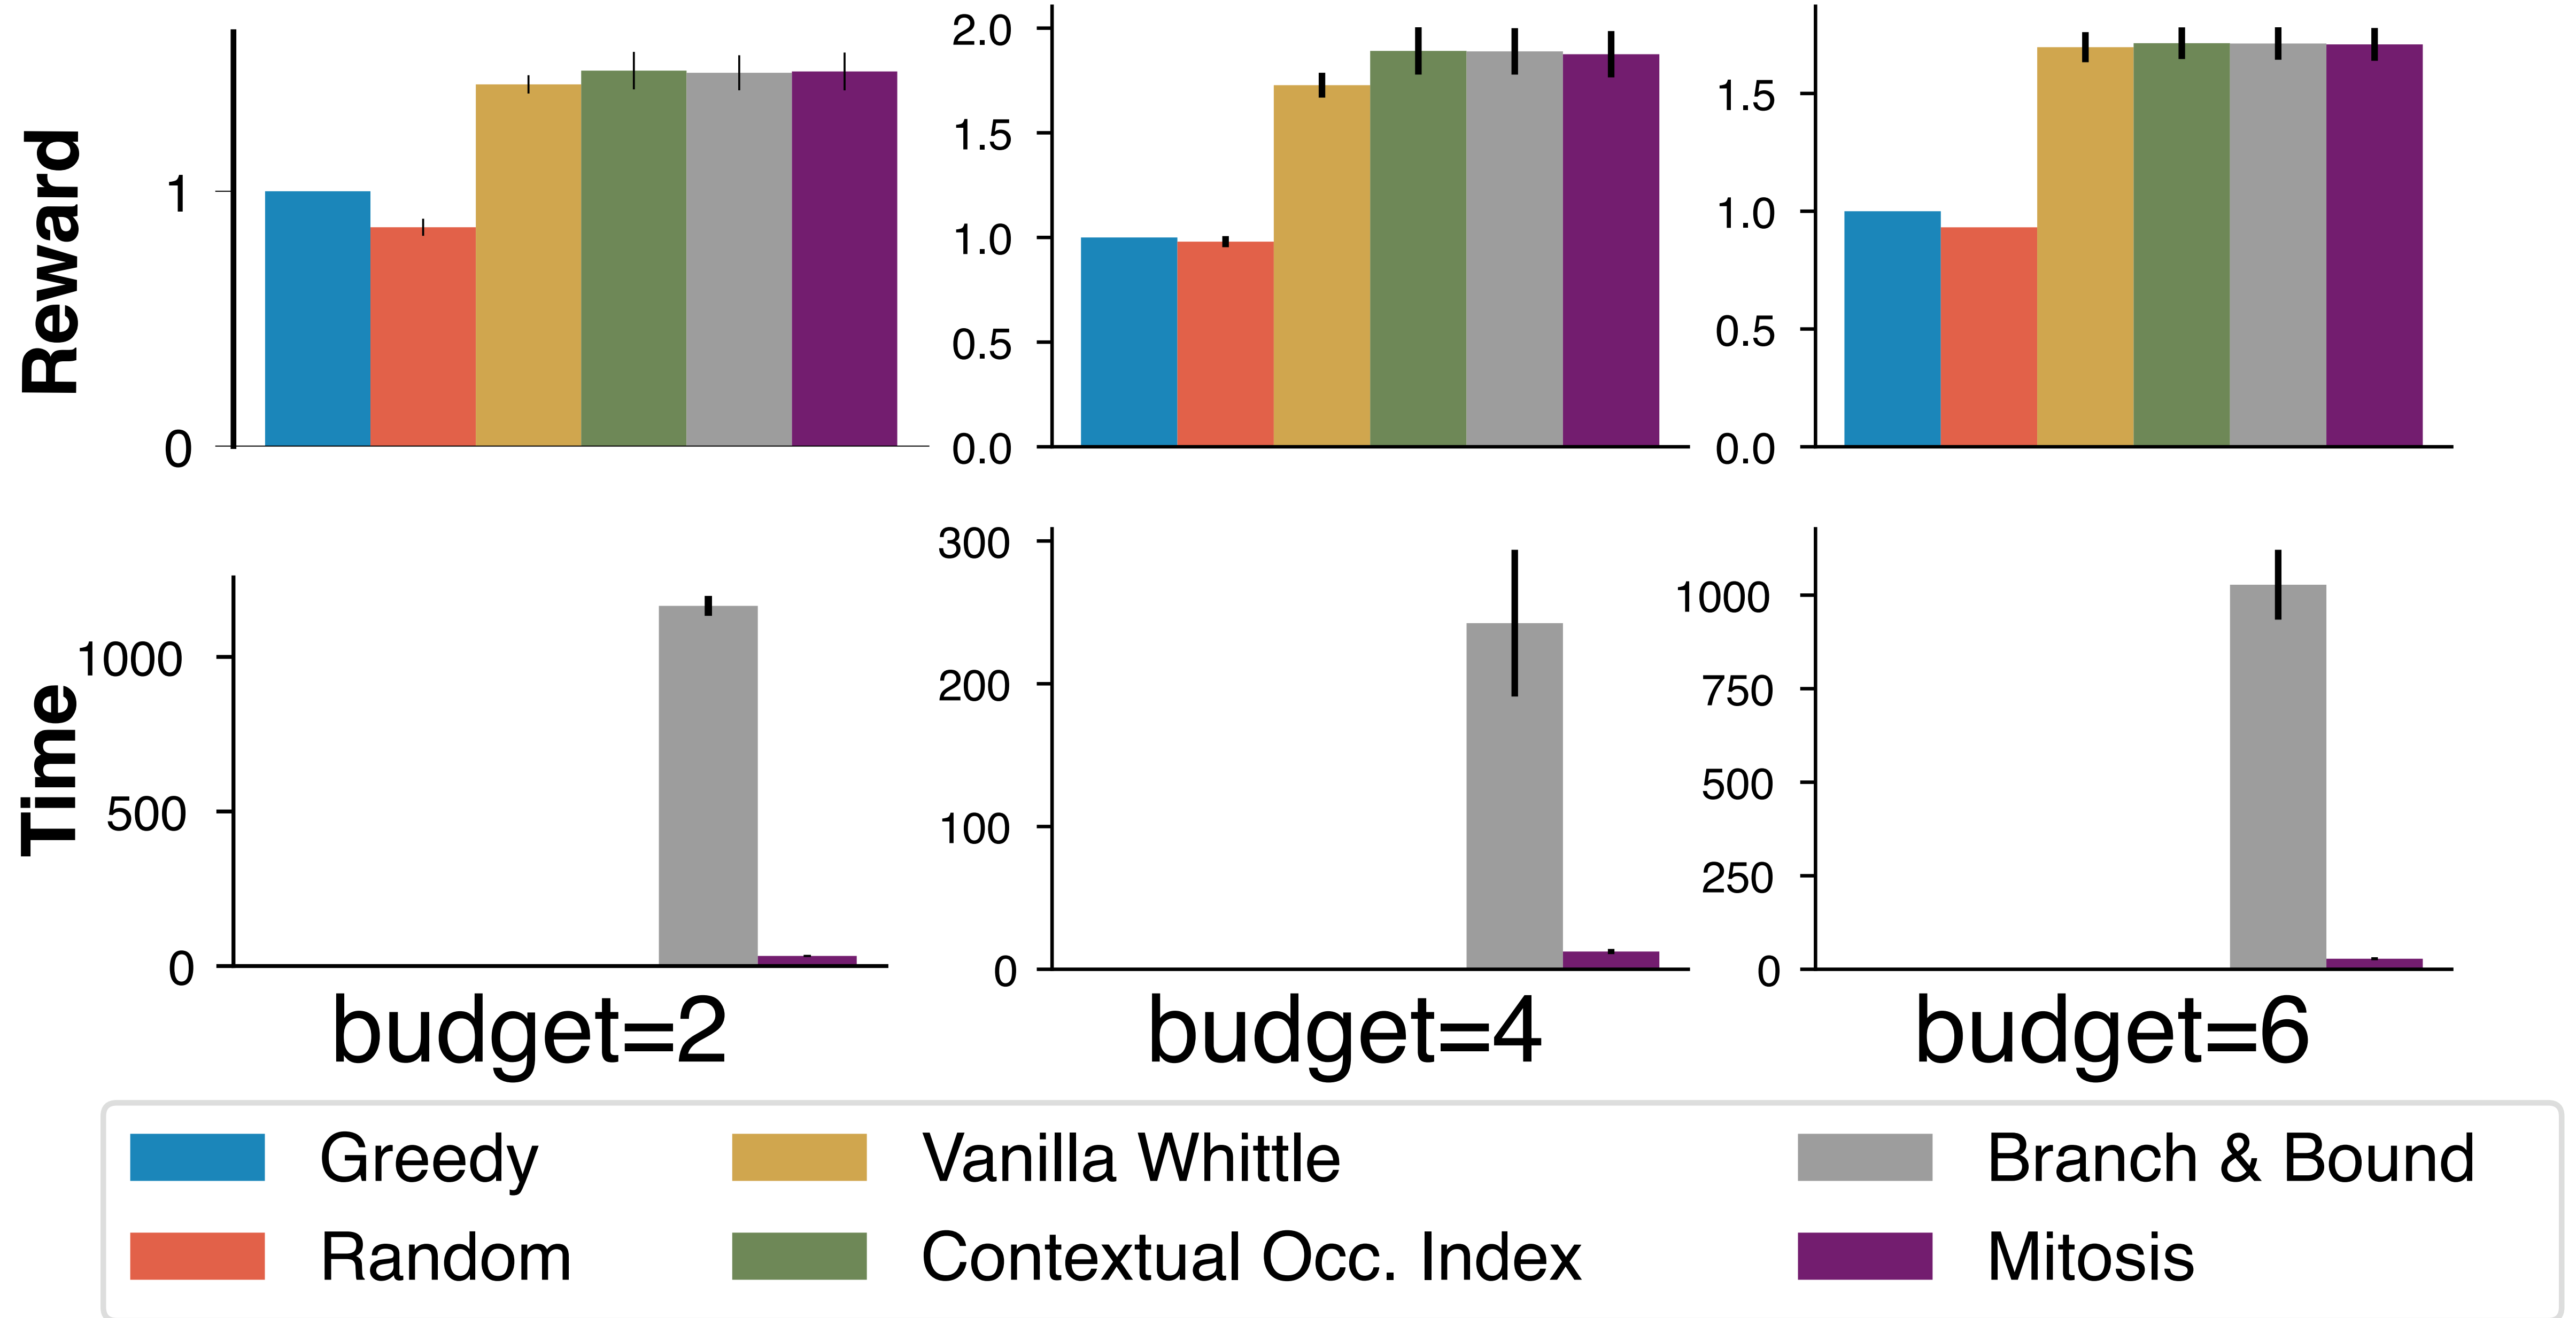

# Synthetic Food Rescue Data

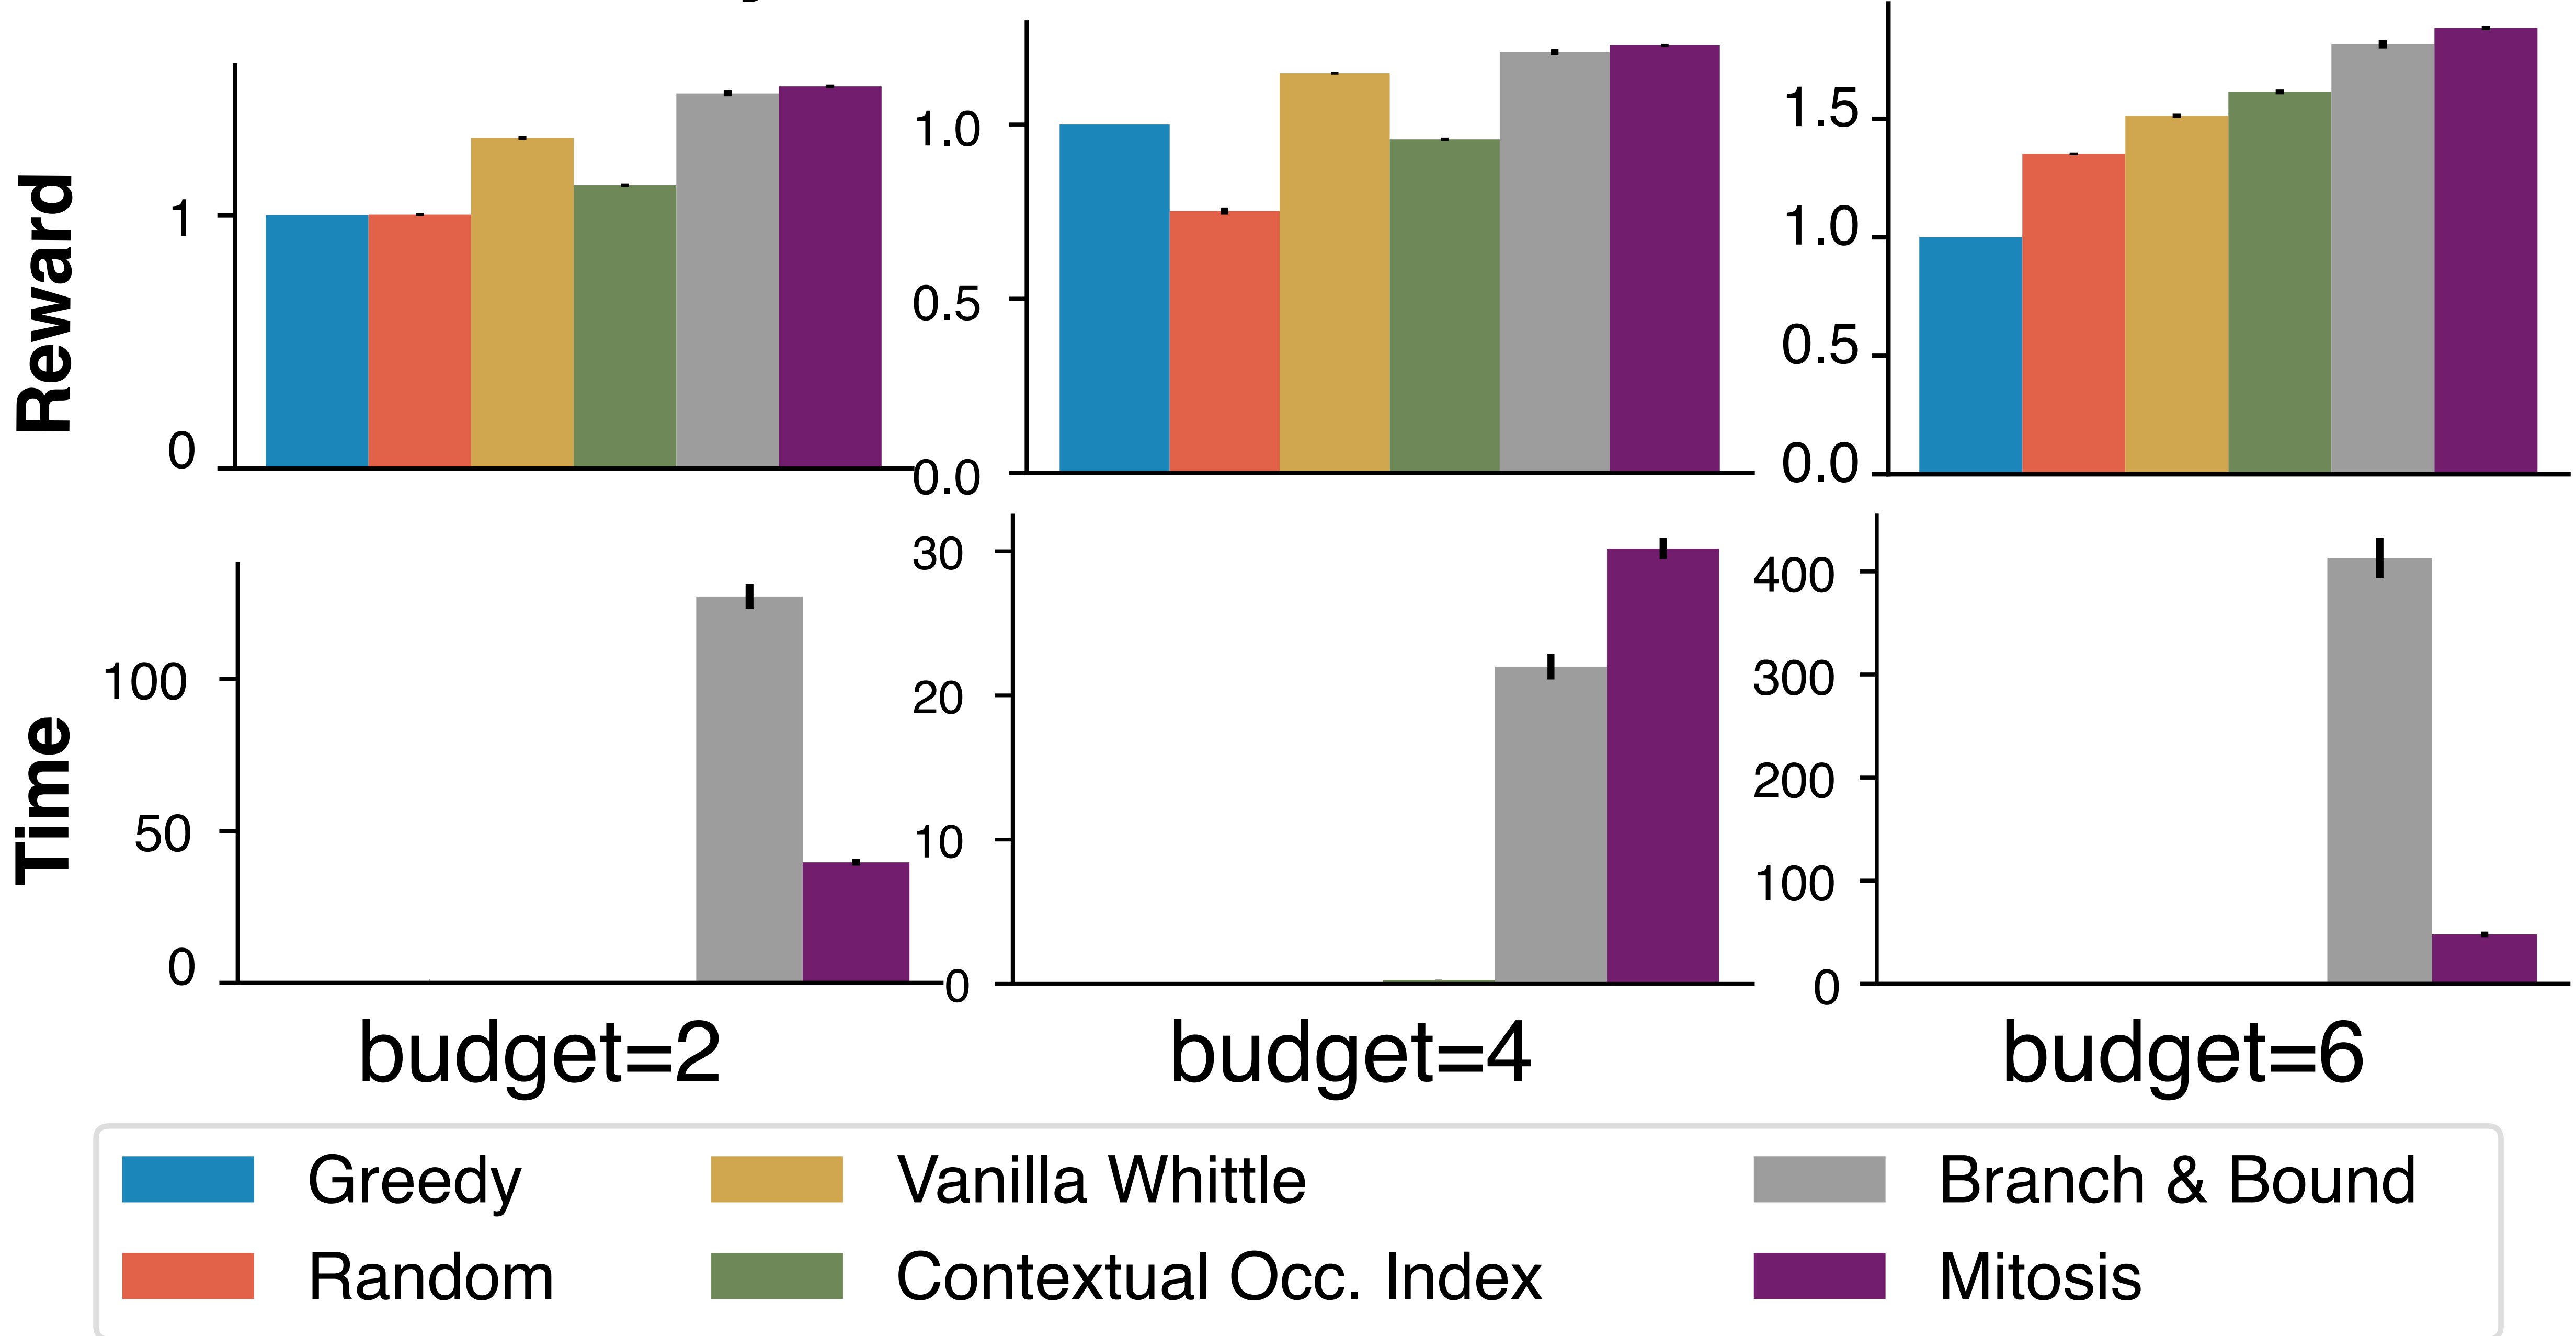

# Real Food Rescue Data

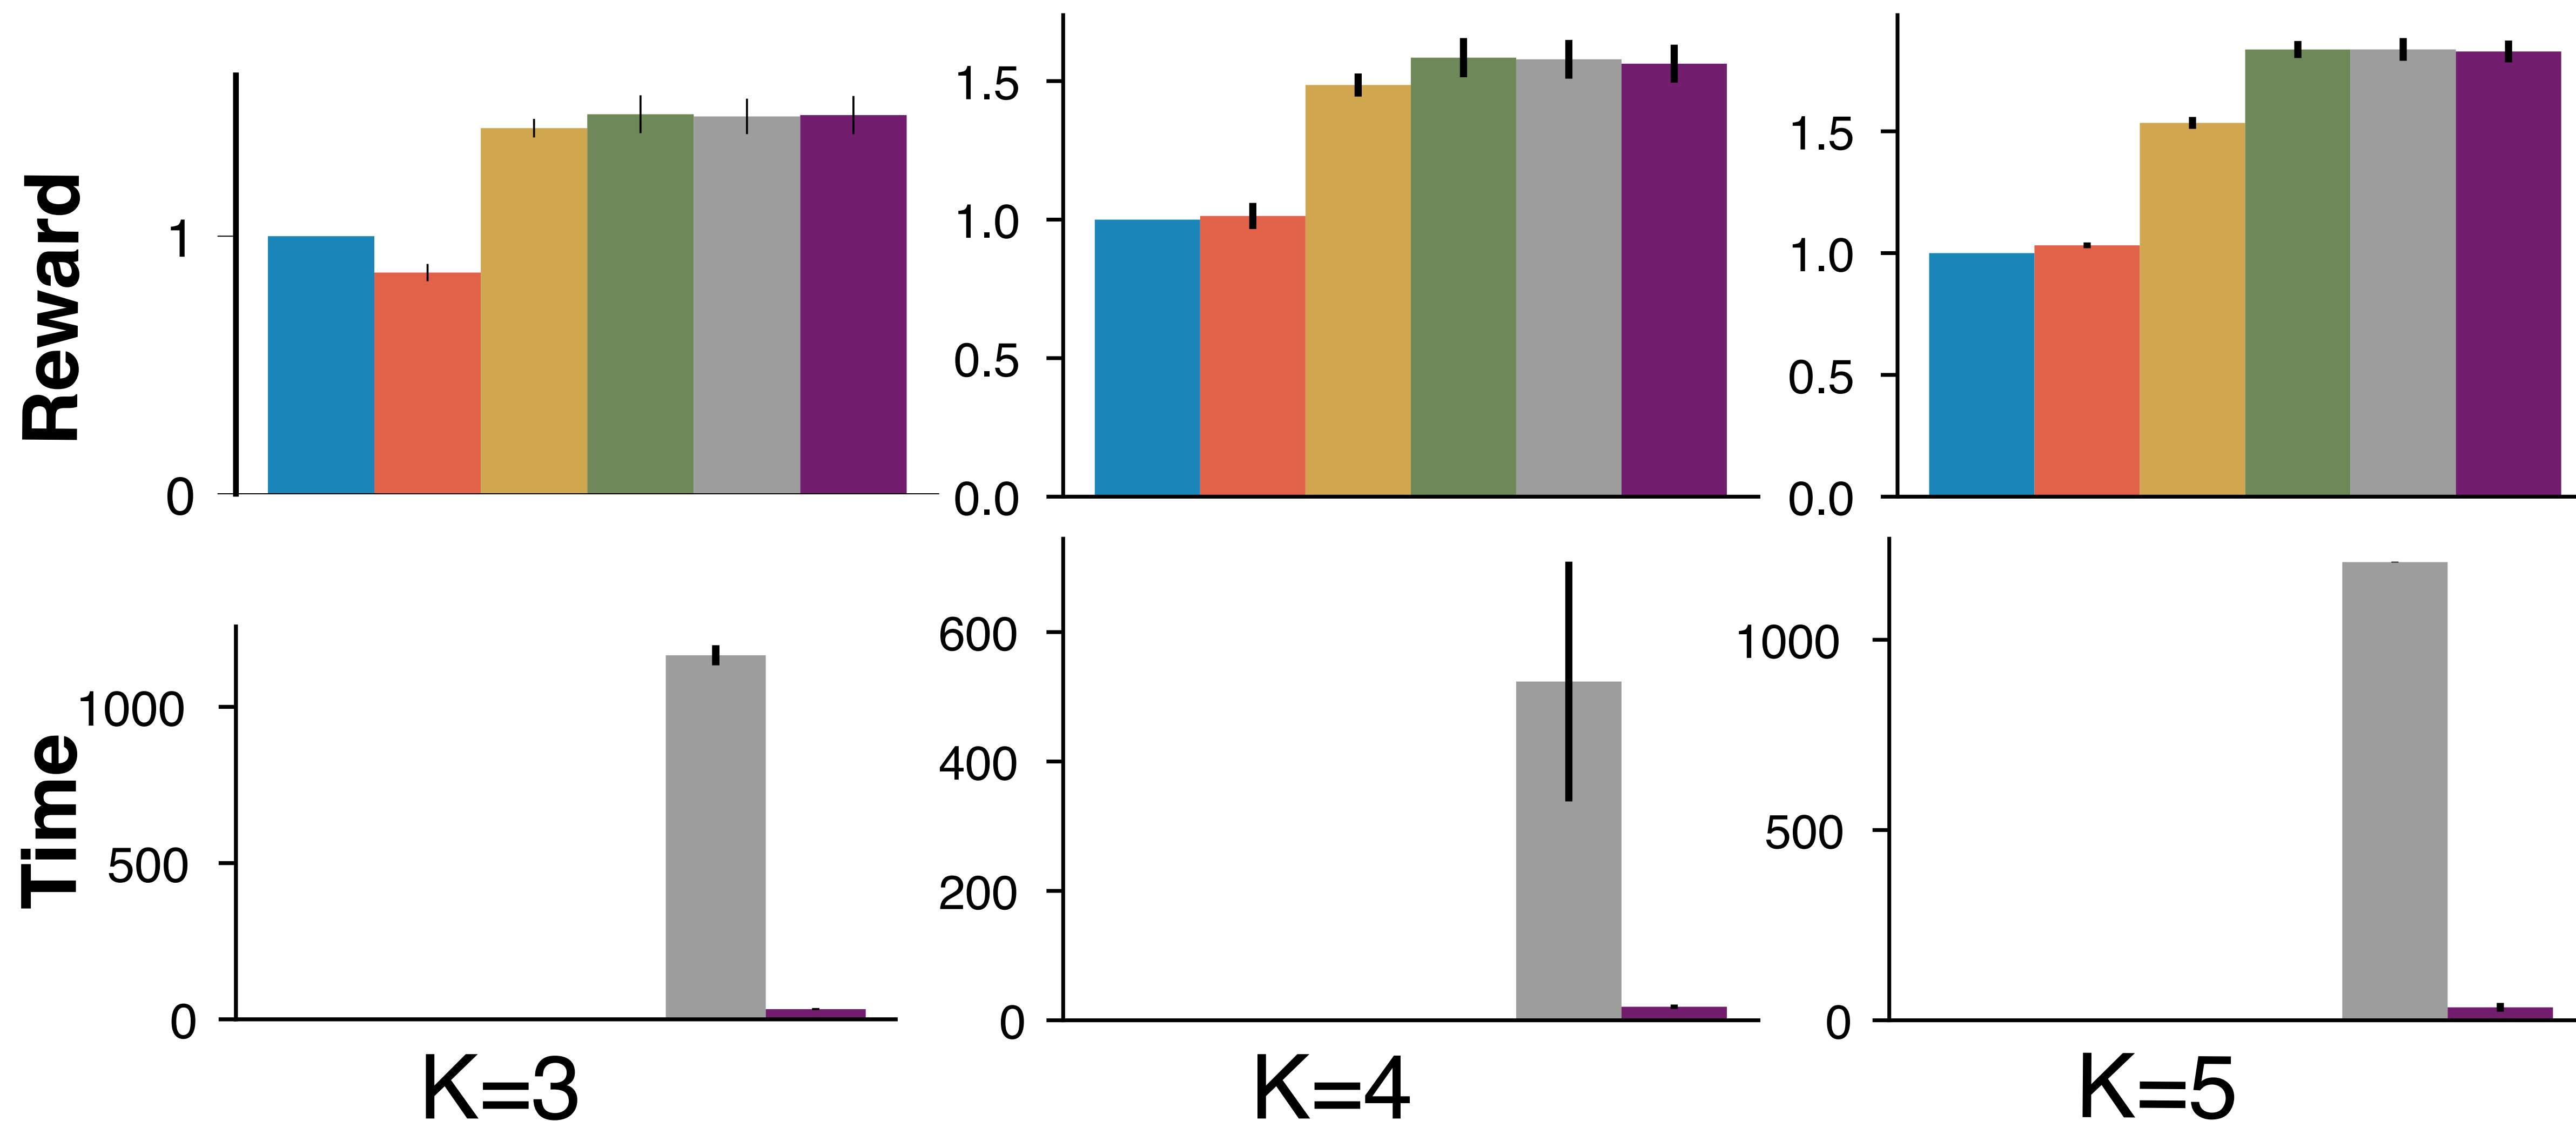

Greedy      Vanilla Whittle      Branch & Bound  
Random      Contextual Occ. Index      Mitosis

# Real Food Rescue Data

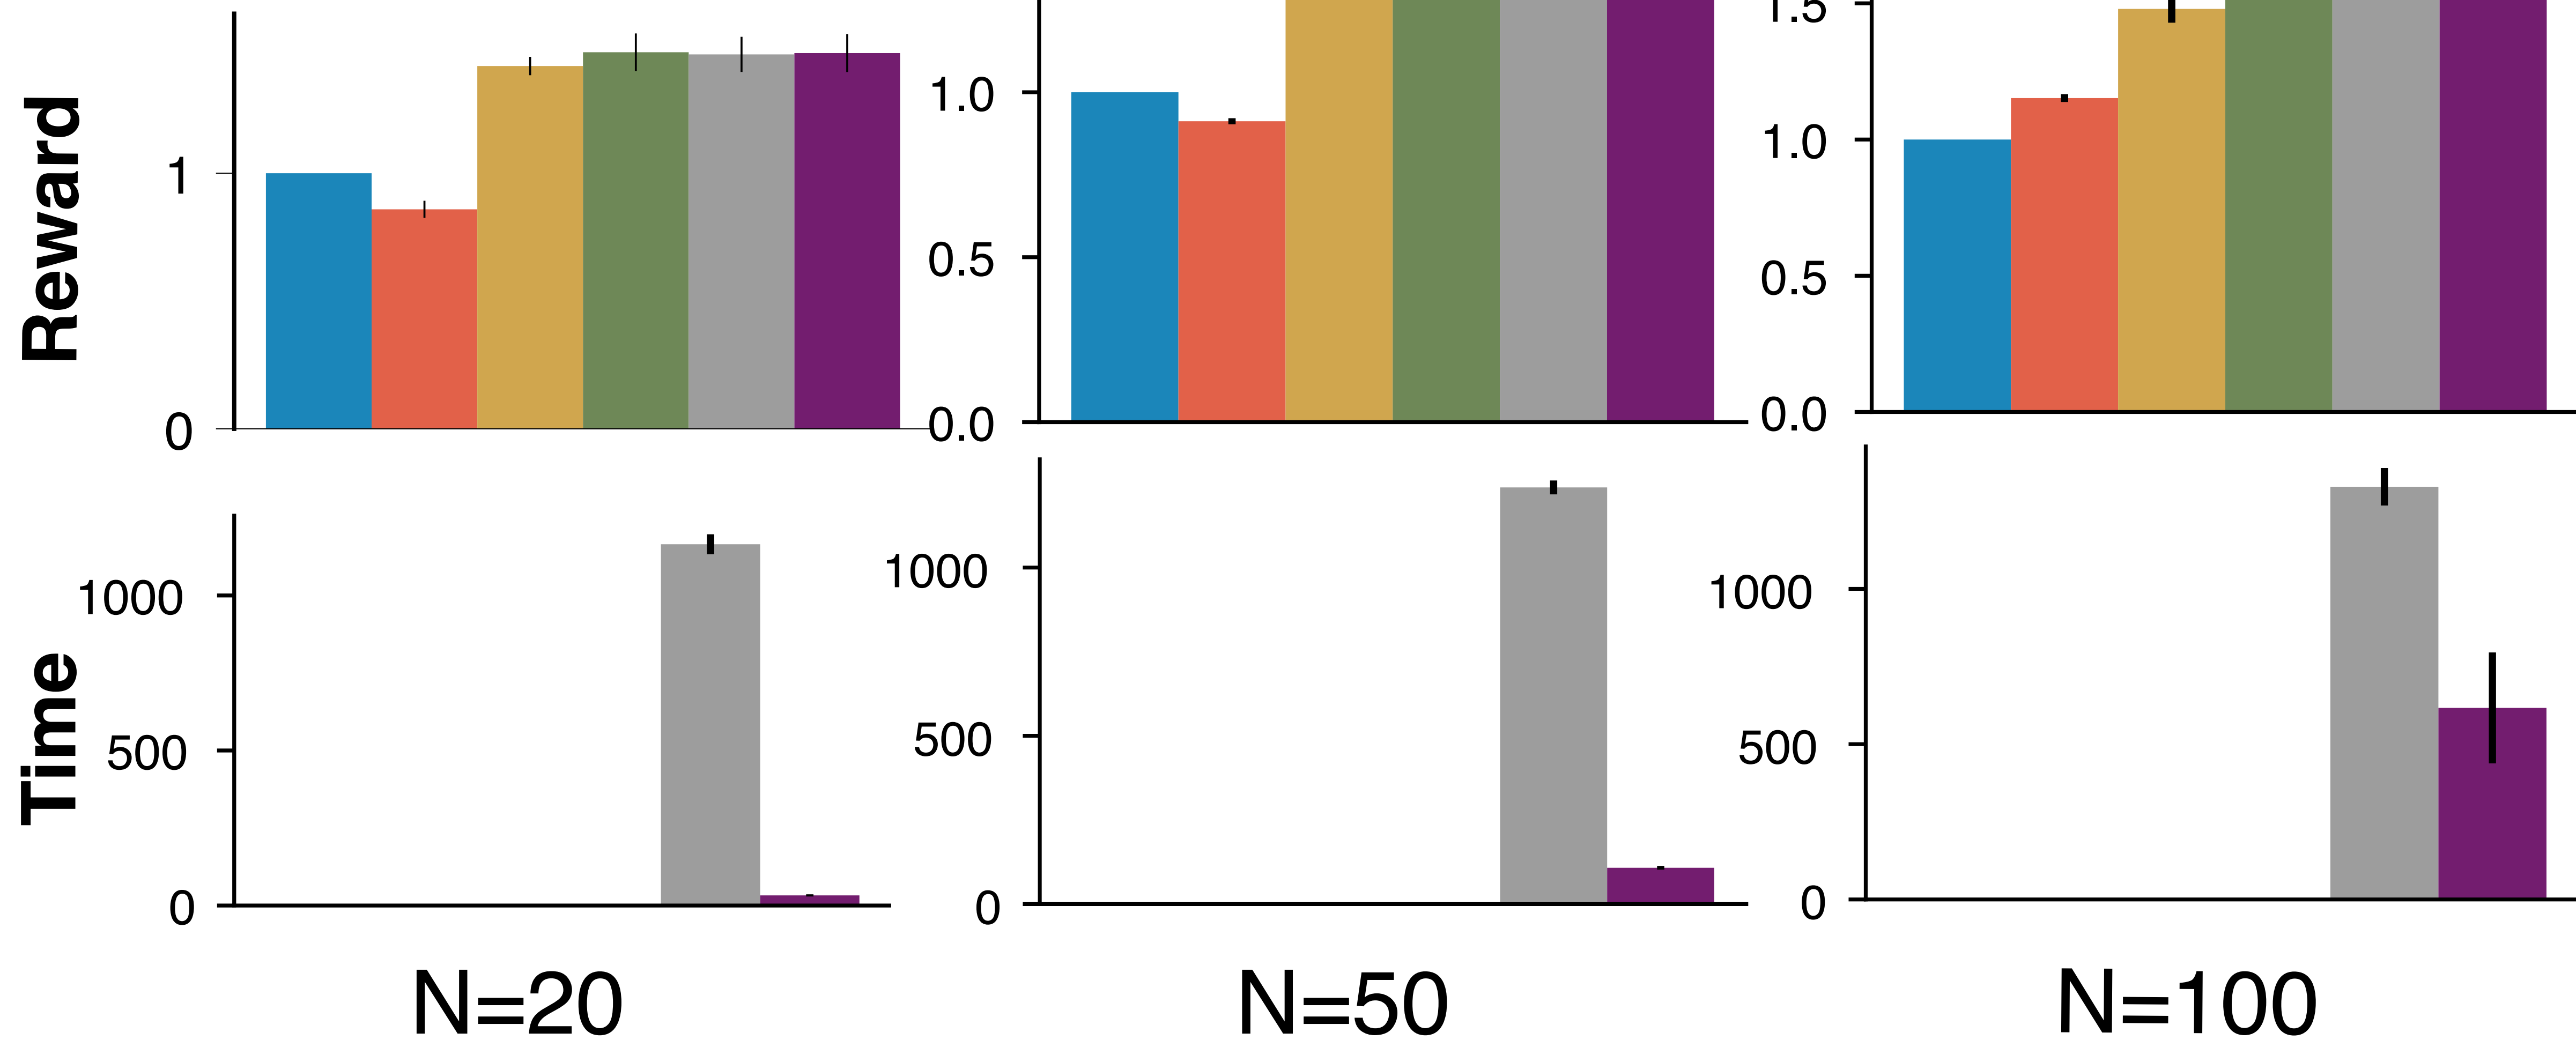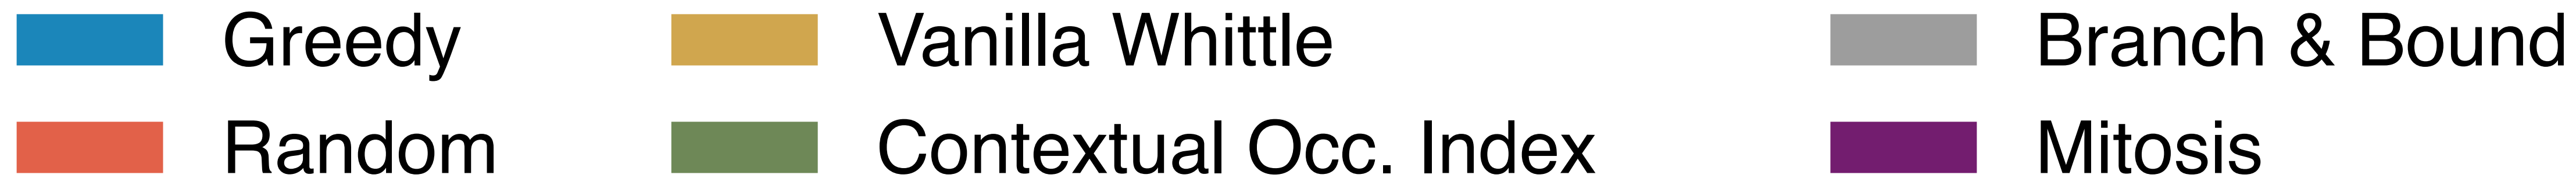

# Synthetic Food Rescue Data

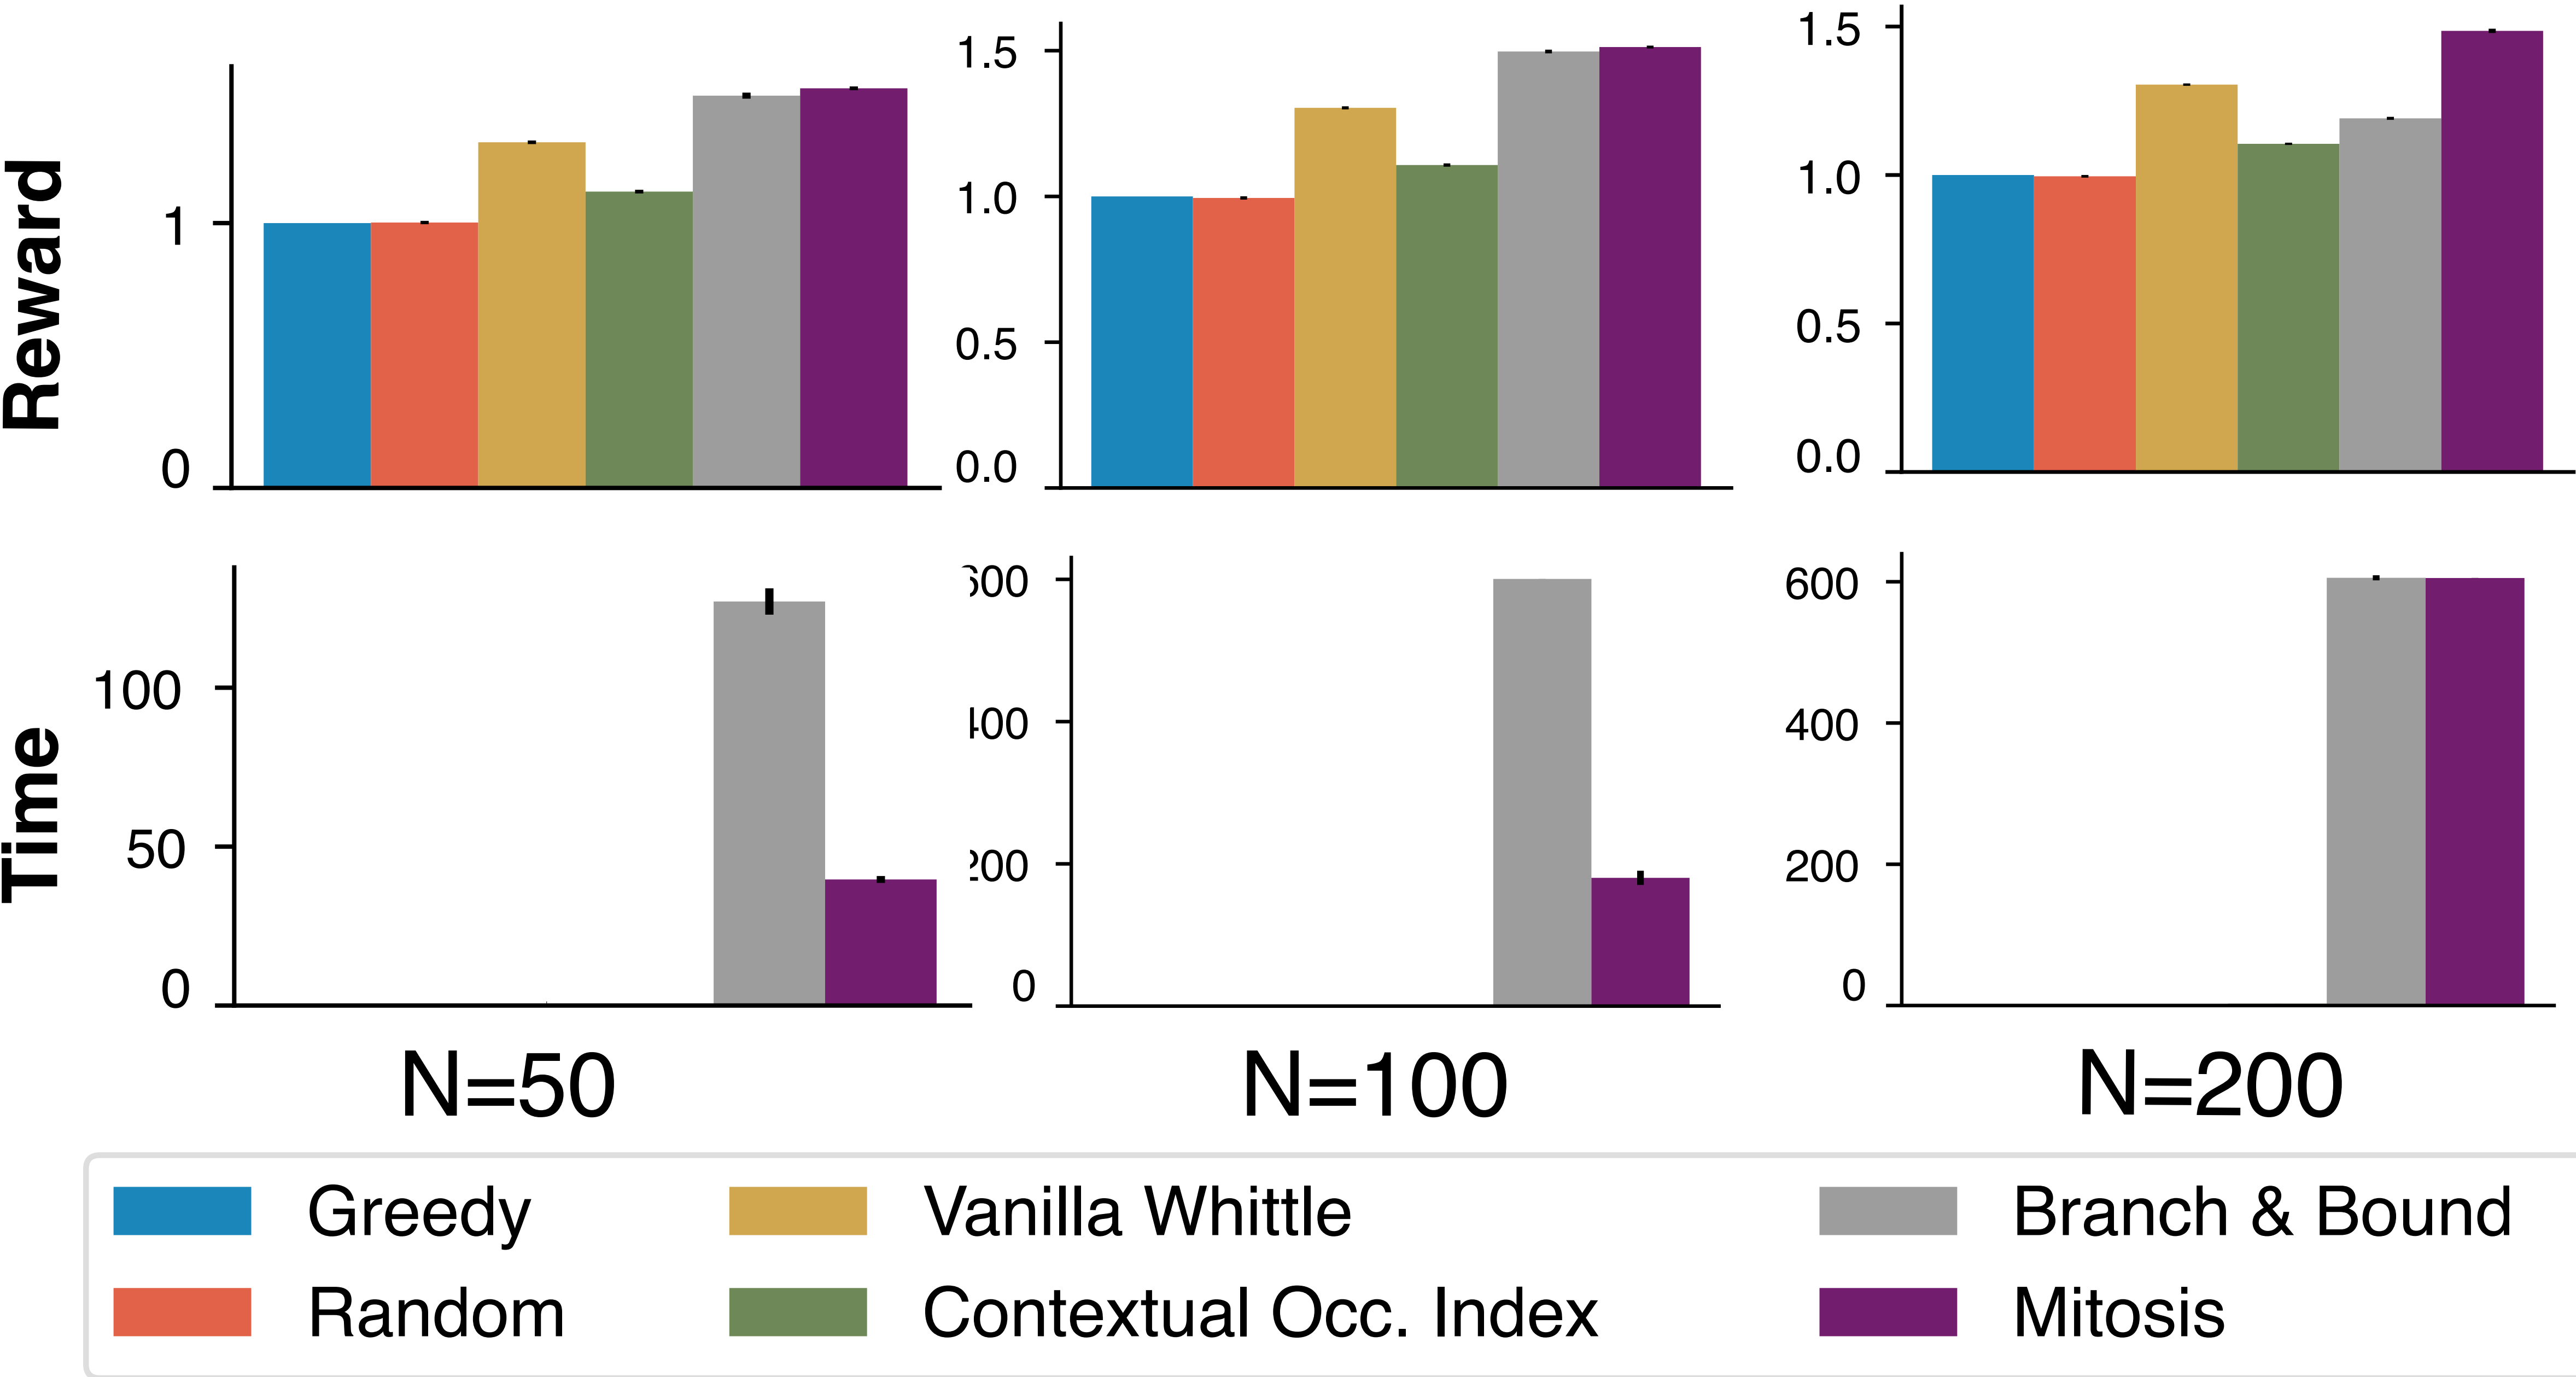

Supplement: Supplementary file 1 [file ablations_appendix.pdf]
